# Supplementary material for: Unanimous Prediction for 100% Precision with Application to Learning Semantic Mappings
Source: arXiv:1606.06368 source file (2016-06-23)
Supplement: Supplementary file 1 [file appendix.tex]

\newpage
\appendix
\section{More extensions} 
\label{App:more_extensions}
In \ref{sec:paraphrasing} we show how to generate some paraphrases for a sentence.
In \ref{sec:partial_mapping} we show how to predict logical form for some part of a sentence when we are not about the whole sentence.

\input{paraphrasing}
\subsection{Partial semantic mappings}
\label{sec:partial_mapping}
\input{partial_recovery_running_examples}
\label{sec:partial_recovery}
Having new word or new combination of words is inevitable in natural language interfaces. In this section we answer this question: how much
of an utterance can we predict subject to 100\% precision?
In our running example (Figure~\ref{fig:sound_parser}), we have three training
inputs and there are only four different mappings
consistent with them (Figure~\ref{fig:atoms_and_mappings}). 
We do not know which one is the correct mapping,
but for some phrases such as: \nl{area of}, \nl{cities in}, \nl{Ohio}, and \nl{Iowa},
all four mappings unanimously agree.
Therefore, we can annotate any of these safe phrases that show up in any utterance.

Given a new utterance $x$,
we enumerate all of $x$'s contiguous phrases $r$
in increasing size and check if $r$ is in $\sFls$,
annotating $r$ with $\ourM(r)$ if it is.
Figure~\ref{fig:partial_recovery_running_examples}
shows how the algorithm treats unseen word or unseen combinations.
\fk{do u think I should explain that we have partial semantic mapping just because $M_{ij} \ge 0$}
